# Supplementary material for: Find the Fungible: Variable-Resolution Tokenization that Compacts Semantics with a Granularity Dial as a VLM "Catalyst"
Source: arXiv:2610.18690 source file (2026-11-24)
Supplement: Supplementary file 1 [file halting_outcomes.tex]

\begin{figure*}[t]
    \centering
    \includegraphics[width=\linewidth]{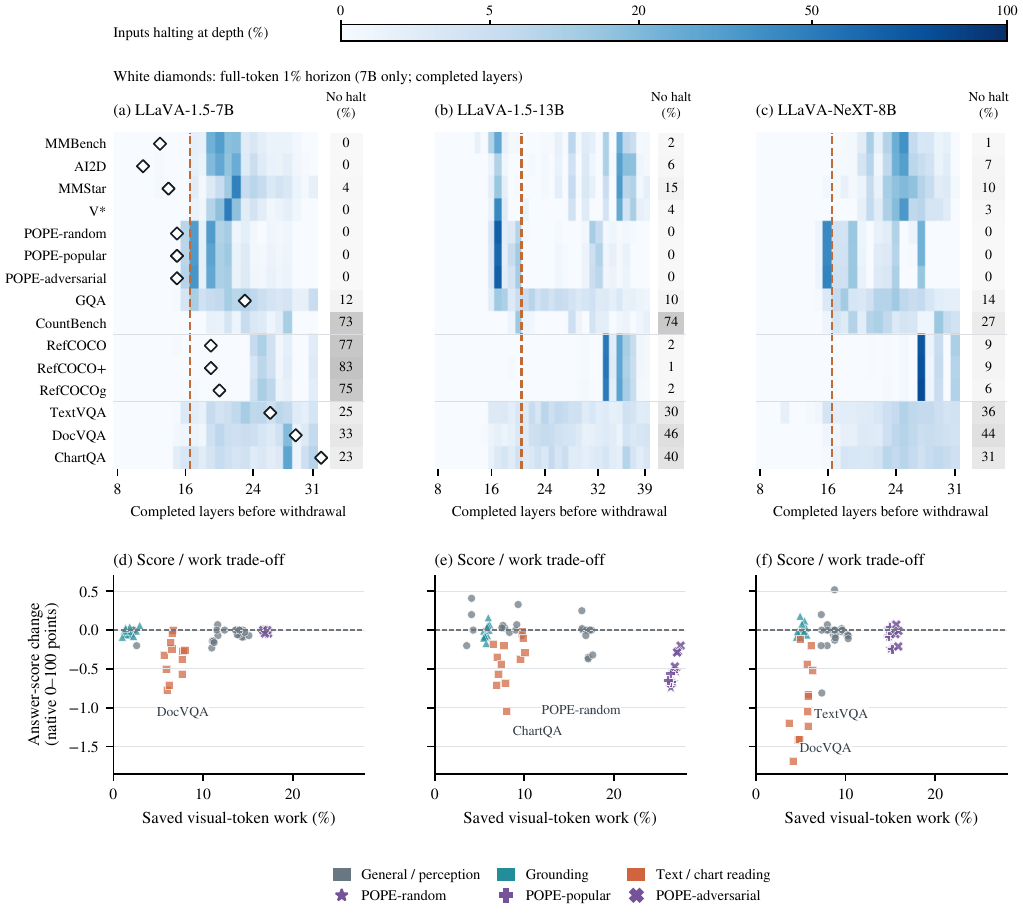}
    \caption{\textbf{Adaptive halting depths versus measured horizons and answer quality.} (a--c) Blue cells give the percentage of all inputs halting at each depth, averaged over four budgets; gray cells give the percentage that never halt. White diamonds in (a) mark the benchmark-level full-token 1\% horizons from Figure~\ref{fig:information_horizon_llava_7}, converted to completed-layer counts. Dashed lines separate halts that bypass \texttt{[REL]} ($h\leq16$ on 7B/NeXT; $h\leq20$ on 13B) from later halts. (d--f) Each point is a metric--budget configuration; negative score changes indicate worse answers. The three POPE splits are shown separately, with distinct purple markers. Saved work is the percentage reduction in image-token processing summed across decoder layers, relative to recorded counts from the matching no-halting run.}
    \label{fig:supp_halting_outcomes}
\end{figure*}
